# Supplementary material for: Time correlations in atmospheric quantum channels
Source: arXiv:2311.07730 ancillary file (2024-07-22)
Supplement: Supplementary file 1 [file Supplement_materials.pdf]

# Time correlations in atmospheric quantum channels: The cases of different channels

M. Klen, D. Vasylyev, W. Vogel, and A. A. Semenov

This supplementary material contains a collection of plots similar to the corresponding plots in the main text of paper, but for several different channels. Here we distinguish three propagation regimes in atmospheric turbulence, characterized by the values of the Rytov parameter: weak impact of turbulence ($\sigma_R^2 < 1$); moderate impact turbulence ($\sigma_R^2 \approx 1$), and strong impact of turbulence ($\sigma_R^2 \gg 1$). For brevity, we refer to these regimes as a to W (weak), M (moderate), and S (strong) regimes. Since the regime of strong impact of turbulence is of great practical interest, three cases are given, denoted as S1, S2, and S3. The following table lists the relevant parameter values used in the simulations:

| Parameter | Weak (W) | Moderate (M) | Strong (S1) | Strong (S2) | Strong (S3) |
|---|---|---|---|---|---|
| Rytov parameter $\sigma_{\mathrm{R}}^2$ | 0.2 | 1.5 | 5.5 | 11 | 16.5 |
| structure constant $C_n^2$ ($\mathrm{m}^{-2/3}$) | $5{\times}10^{-15}$ | $1.5{\times}10^{-14}$ | $1{\times}10^{-16}$ | $2{\times}10^{-16}$ | $3{\times}10^{-16}$ |
| outer scale $L_0$ (m) | 80 | 80 | 80 | 80 | 80 |
| inner scale $\ell_0$ (m) | $10^{-3}$ | $10^{-3}$ | $10^{-3}$ | $10^{-3}$ | $10^{-3}$ |
| channel length $z_{\mathrm{ap}}$ (km) | 1 | 1.6 | 50 | 50 | 50 |
| beam-spot radius at the transmitter, $W_0$ (cm) | 2 | 2 | 8 | 8 | 8 |
| wavelength $\lambda = 2\pi/k$ (nm) | 809 | 809 | 808 | 808 | 808 |

## I. CONDITIONAL PDT

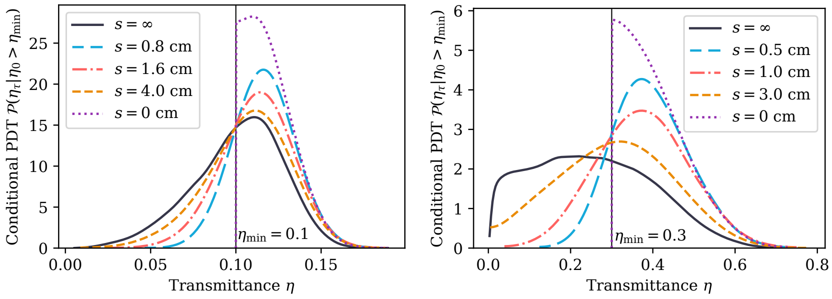


Figure 1. The channel W with $R_{\mathrm{ap}} = 0.35$ cm and the channel M with $R_{\mathrm{ap}} = 1.4$ cm (left and right plots, respectively).

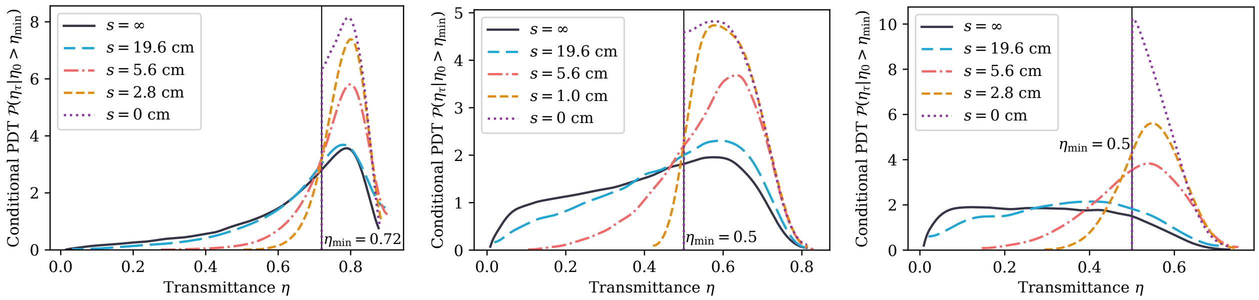


Figure 2. The channels S1, S2, and S3 with $R_{\mathrm{ap}} = 30$ cm (from left to right).

## II. SPATIAL COHERENCE RADIUS VS APERTURE RADIUS

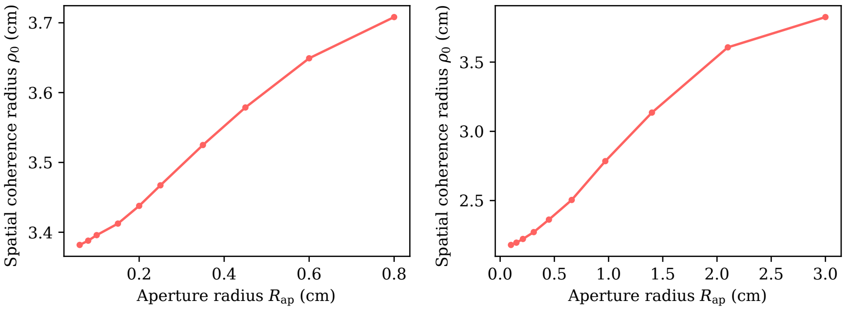


Figure 3. The channel W and the M (left and right plots, respectively).

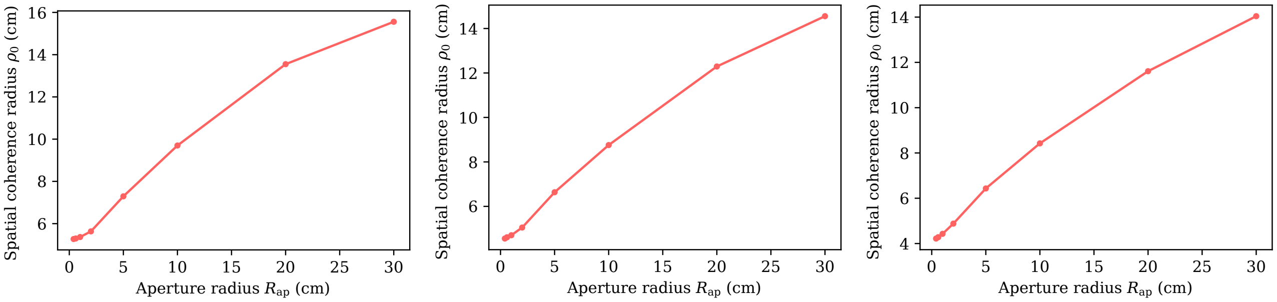


Figure 4. The channels S1, S2, and S3 (from left to right).

## III. GAUSSIAN ENTANGLEMENT: SIMON CERTIFIER ON THE PLANE WIND-DRIVEN SHIFT — SQUEEZING PARAMETER

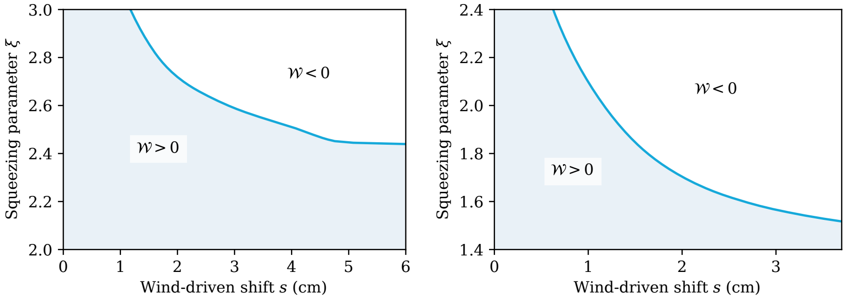


Figure 5. The squeezing parameter $\xi$ vs. the wind-driven shift $s$ for the value of the Simon certifier $W = 0$ is shown for the channel W with $R_{\mathrm{ap}} = 0.35$ cm and the channel M with $R_{\mathrm{ap}} = 0.97$ cm (left and right plots, respectively). The hatched areas correspond to the domains, where Gaussian entanglement is preserved.

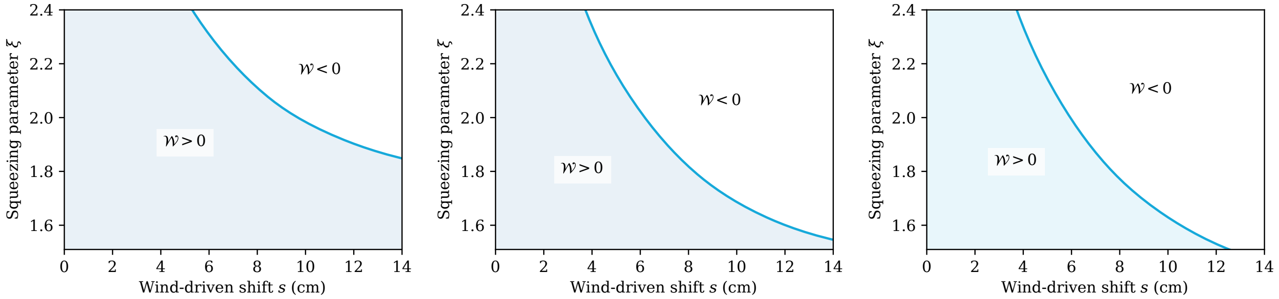


Figure 6. The same as on the above figure but for the channels S1, S2, and S3 with $R_{\mathrm{ap}} = 20$ cm from left to right, respectively .

## IV. GAUSSIAN ENTANGLEMENT: THRESHOLD WIND-DRIVEN SHIFT VS SPATIAL COHERENCE RADIUS

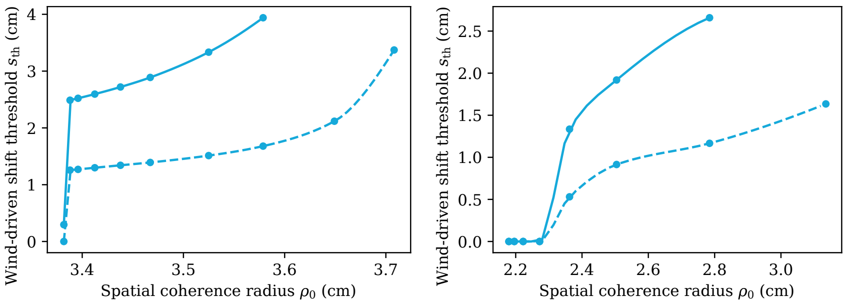


Figure 7. The channel W (the left plot, the solid and dashed lines correspond to $\xi = 2.5$ and $\xi = 2.9$, respectively) and the channel M (the right plot, the solid and dashed lines correspond to $\xi = 1.6$ and $\xi = 2$, respectively) .

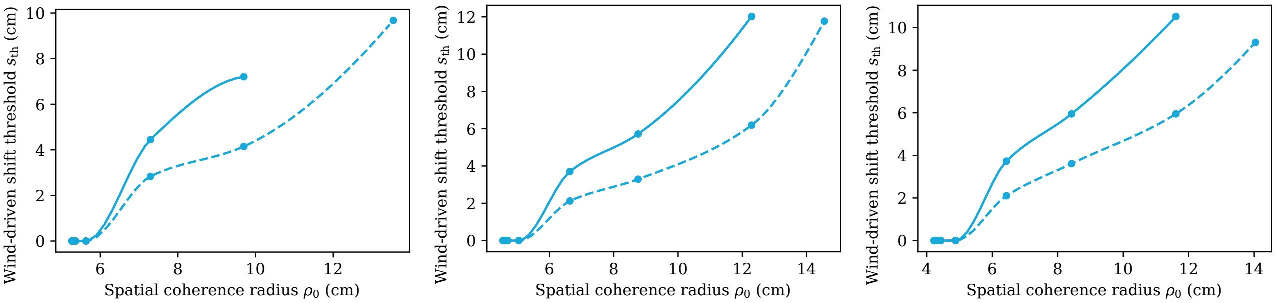


Figure 8. The channels S1, S2, and S3 (the left plot, the solid and dashed lines correspond to $\xi = 1.6$ and $\xi = 2$, respectively) from left to right.

## V. DISCRETE-VARIABLE ENTANGLEMENT: BELL PARAMETER VS TIME BETWEEN ENTANGLED PULSES

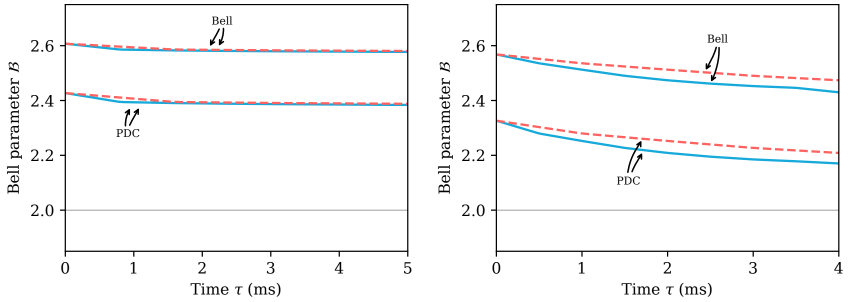


Figure 9. The channel W (left plot) with $R_{\rm ap} = 0.25$ cm and the channel M (right plot) with $R_{\rm ap} = 0.45$ cm for the Bell-state and the PDC state. The mean number of noise counts in both cases is $5 \times 10^{-4}$. The solid and dashed lines correspond to the wind velocity $v = 10$ m/s and $v = 5$ m/s, respectively. Quantum memory is considered to be lossless.

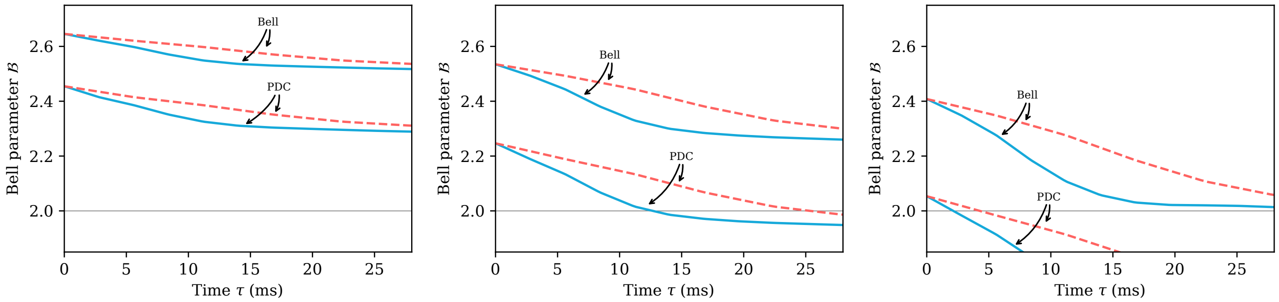


Figure 10. The same as on the figure above but for the channels S1, S2, and S3 with $R_{\rm ap} = 10$ cm.

## VI. ADAPTIVE REAL-TIME SELECTION FOR NONCLASSICAL STATES

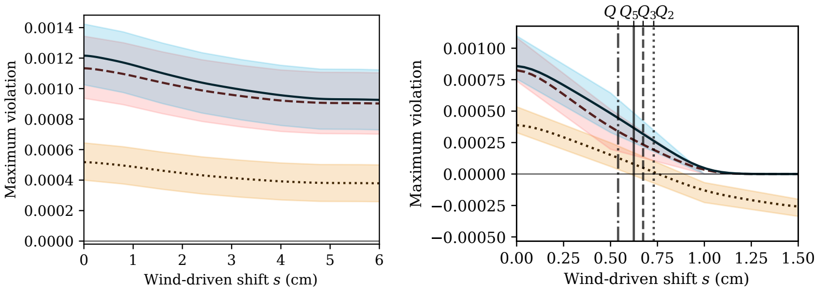


Figure 11. Maximum violation of inequality $\sum_{n=0}^{N-1}\lambda(n)P(n)\leq\sup_{\alpha\in\mathbb{C}}\sum_{n=0}^{N-1}\lambda(n)\Pi(n|\alpha)$ for click detectors vs the wind-driven shift $s$ for the amplitude-squeezed state with $\alpha_0=1.15$ and $\xi=0.59$. The left and right plots correspond to the channel W with $R_{\rm ap}=0.35$ cm and $\eta_{\rm min}=0.04$ and the channel M with $R_{\rm ap}=0.45$ cm and $\eta_{\rm min}=0.055$, respectively. The symbols $Q$ and $Q_N$ indicate the thresholds of $s$ for which $Q=0$ (dash-dotted line) and $Q_N=0$, respectively. The dotted, dashed, and solid vertical lines and curves correspond to $N=2$, $N=3$, and $N=5$, respectively. The overall deterministic losses are 6 dB.

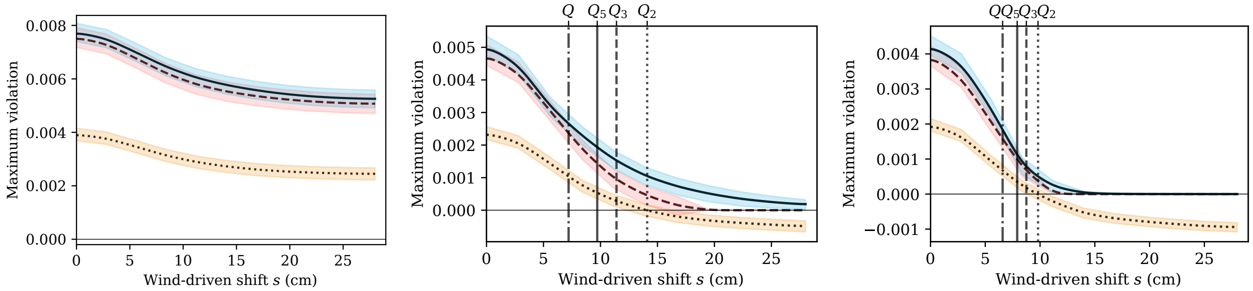


Figure 12. The same as on the figure above but for the channels S1, S2, and S3 with $R_{\rm ap}=30$ cm and $\eta_{\rm min}=0.1$.
